# Supplementary material for: TCFormer: Visual Recognition via Token Clustering Transformer
Source: arXiv:2407.11321 source file (2024-07-16)
Supplement: Supplementary file 1 [file appendix.tex]

\section{Dynamic Tokens}
We show more examples of the vision token generated by our TCFormer on various tasks in Fig.~\ref{fig:token_vis_appendix}. To clearly demonstrate the focus of our dynamic tokens, we visualize the density of tokens, which is inversely proportional to the image region represented by the token.

These examples further validate the advantages of our dynamic tokens in all tasks. Firstly, the dynamic tokens align well with the objects in images, see the left top examples in Fig.~\ref{fig:token_vis_appendix}(a) and Fig.~\ref{fig:token_vis_appendix}(d).
Secondly, the TCFormer allocates more tokens to the valuable regions and represents 
the uninformative regions with a few tokens, which can be visualize from the token density maps.
Thirdly, intricate image details are represented by fine tokens, \ie the boat in the boat in the bottom right example of Fig.~\ref{fig:token_vis_appendix}(a), the hands in Fig.~\ref{fig:token_vis_appendix}(b), the windows in the top left example of Fig.~\ref{fig:token_vis_appendix}(c).

The good properties of the dynamic tokens in all tasks proves the versatility of our TCFormer.

Additional examples of the vision tokens generated by TCFormer on various tasks can be seen in Fig.~\ref{fig:token_vis_appendix}. To highlight the focus of our dynamic tokens, we visualize the token density, which is inversely proportional to the region of the image represented by the token. These examples further affirm the benefits of our dynamic tokens in all tasks. Firstly, the dynamic tokens align well with the objects in the images, as seen in the top left examples of  Fig.~\ref{fig:token_vis_appendix}(a) and Fig.~\ref{fig:token_vis_appendix}(d). Secondly, TCFormer allocates more tokens to the informative regions and represents the less significant regions with a small number of tokens, which can be observed in the token density maps. Thirdly, valuable image details are represented by finer tokens, such as the boat in the bottom right example of Fig.~\ref{fig:token_vis_appendix}(a), the human hands in Fig.~\ref{fig:token_vis_appendix}(b), and the windows in the top left example of Fig.~\ref{fig:token_vis_appendix}(c). The beneficial attributes of the dynamic tokens in a range of tasks illustrate the flexibility of TCFormer across various applications.

\begin{figure*}[tb]
	\centering
	\includegraphics[width=0.98\textwidth]{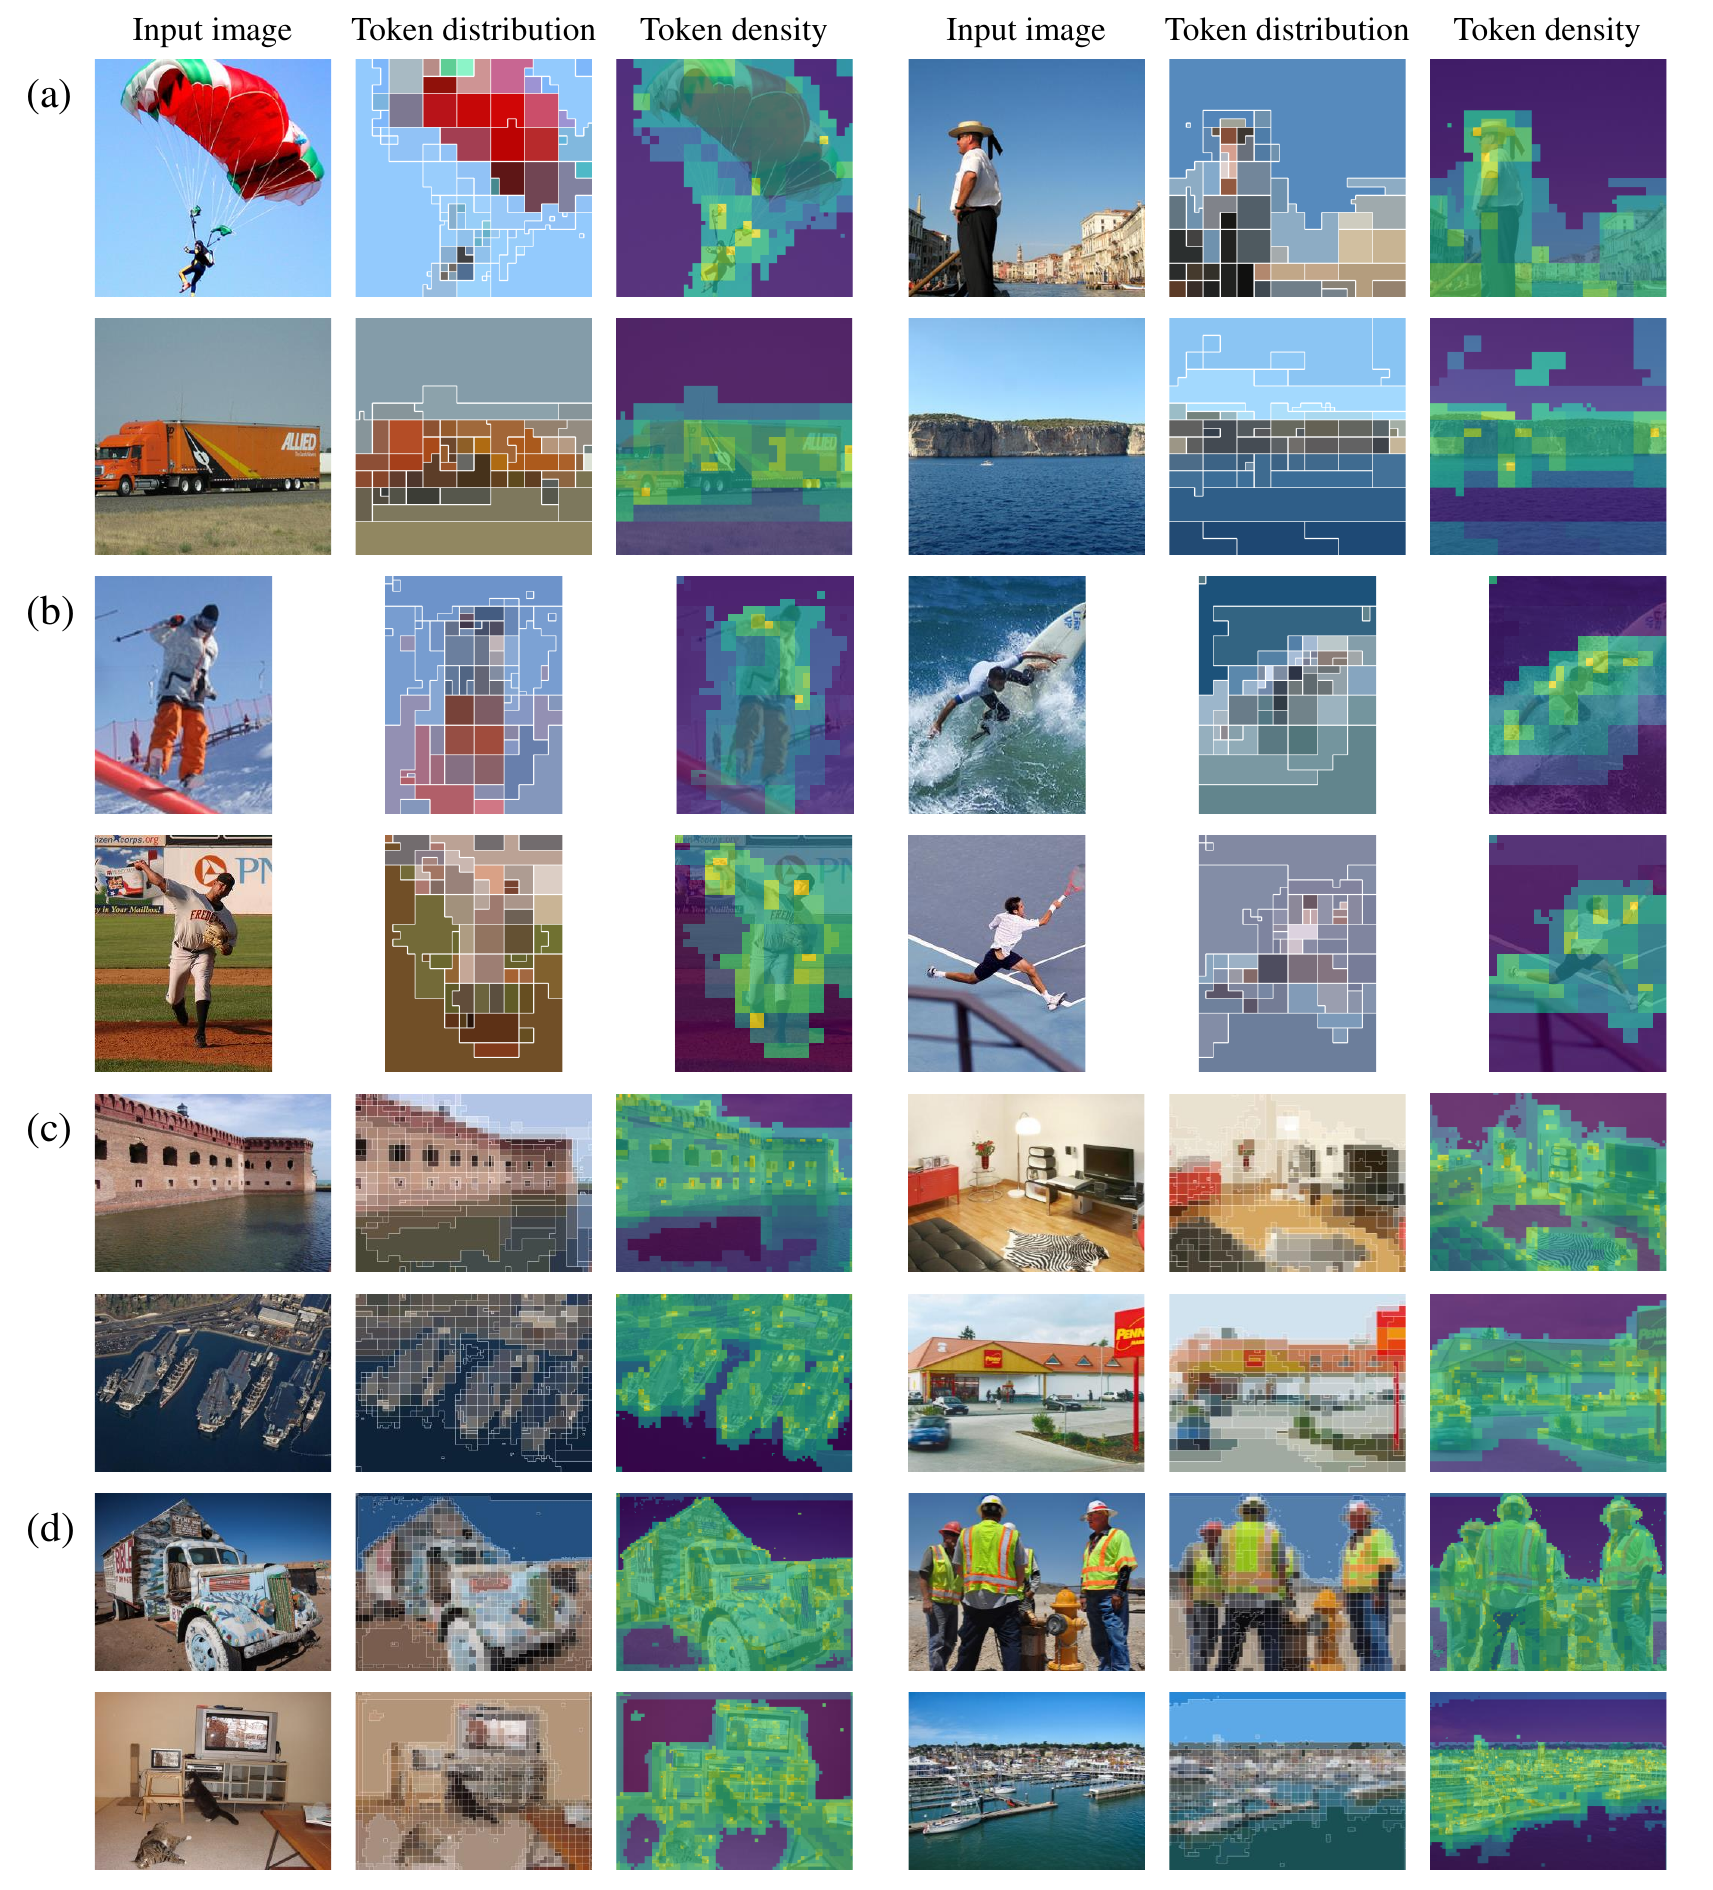}
        \caption{
        Examples of the dynamic vision tokens generated by TCFormer on (a) image classification, (b) human pose estimation, (c) semantic segmentation and (d) object detection.
        }
	\label{fig:token_vis_appendix}
\end{figure*}
